# Supplementary material for: Safe Control of Partially-Observed Linear Time-Varying Systems with Minimal Worst-Case Dynamic Regret
Source: arXiv:2208.08929 source file (2023-03-31)
Supplement: Supplementary file 1 [file 0-Supplementary.tex]

\vspace{-6mm}
\section*{Supplementary Material}\label{sec:sup}
% \begin{itemize}[leftmargin=9pt]
    % \item 
    {In the arXiv version of this paper~\cite{zhou2022safe}, we also include a trajectory tracking scenario of a hovering quadrotor collecting GPS and Inertial Measurement Unit (IMU) measurements.}
% \end{itemize}
